# Supplementary material for: Hyper-Bagel: A Unified Acceleration Framework for Multimodal Understanding and Generation
Source: arXiv:2509.18824 source file (2025-09-23)
Supplement: Supplementary file 1 [file appendix.tex]

\section{Hello World}
%\subsection{Hello World}
